# Supplementary material for: Universality of the collapse transition of sticky polymers
Source: arXiv:1903.07356 ancillary file (2019-09-02)
Supplement: Supplementary file 1 [file supp_info.pdf]

**Supplementary Information for:**

# Universality of the collapse transition of sticky polymers

Aritra Santra,[1] Kiran Kumari,[2,3,1] R. Padinhateeri,[3] B. Dünweg,[4,1] and J. Ravi Prakash[1,a)]

[1)] *Department of Chemical Engineering, Monash University, Melbourne, VIC 3800, Australia*

[2)] *IITB-Monash Research Academy, Indian Institute of Technology Bombay, Mumbai, Maharashtra - 400076, India*

[3)] *Department of Biosciences and Bioengineering, Indian Institute of Technology Bombay, Mumbai, Maharashtra - 400076, India*

[4)] *Max Plank Institute of Polymer Research, Ackermannweg 10, 55128 Mainz, Germany*

[a)] Electronic mail: ravi.jagadeeshan@monash.edu

## I. The cut-off radius for the SDK potential

As was pointed out in the main text, in the original study by Soddemann et al.[1] the cut-off radius of the SDK potential, $r_c$, was chosen to be $1.5\,\sigma$ in order to include only the first neighboring shell of interactions, determined from the first minimum of the pair correlation function. In this supplementary information, we first show that in the context of the Brownian dynamics simulations carried out in this work, the choice of $r_c = 1.5\,\sigma$ leads to the prediction of unphysical asymptotic scaling behaviour in the poor solvent limit. We then discuss how an appropriate value of the cut-off radius can be estimated. For the sake of completeness and clarity, we repeat some of the equations that have already been displayed in the main text.

The potential proposed by Soddemann-Dünweg-Kremer (SDK)[1] has the form,

$$U_{\mathrm{SDK}} = \begin{cases} 4\left[\left(\dfrac{\sigma}{r}\right)^{12} - \left(\dfrac{\sigma}{r}\right)^{6} + \dfrac{1}{4}\right] - \epsilon; & r \leq 2^{1/6}\sigma \\ \dfrac{1}{2}\epsilon\left[\cos\left(\alpha\left(\dfrac{r}{\sigma}\right)^{2} + \beta\right) - 1\right]; & 2^{1/6}\sigma \leq r \leq r_c \\ 0; & r \geq r_c \end{cases} \tag{1}$$

A comparison is drawn in Fig. S1 between the SDK potential and the conventional Lennard-Jones (LJ) and Weeks-Chandler-Andersen (WCA) potentials, the expressions of which are given in Eq. (2) and Eq. (3), respectively.

$$U_{\mathrm{LJ}} = 4\epsilon_{\mathrm{LJ}}\left[\left(\frac{\sigma}{r}\right)^{12} - \left(\frac{\sigma}{r}\right)^{6}\right] \tag{2}$$

$$U_{\mathrm{WCA}} = \begin{cases} 4\epsilon_{\mathrm{LJ}}\left[\left(\dfrac{\sigma}{r}\right)^{12} - \left(\dfrac{\sigma}{r}\right)^{6} + \dfrac{1}{4}\right]; & r \leq 2^{1/6}\sigma \\ 0; & r > 2^{1/6}\sigma \end{cases} \tag{3}$$

In the above equations, $\sigma$ is the non-dimensional distance at which the LJ potential becomes zero, and its value is taken to be 1 in the present study. The quantities $\epsilon$ and $\epsilon_{\mathrm{LJ}}$ are the attractive well depths of the SDK and LJ potentials, respectively. As shown in Fig. S1, unlike the LJ potential, which has a long attractive tail, the short ranged attractive tail of the SDK potential smoothly approaches zero at a finite distance $r_c$. The choice $\epsilon = 0$ in the SDK potential is equivalent to $\epsilon_{\mathrm{LJ}} = 1.0$ in the purely repulsive WCA potential.

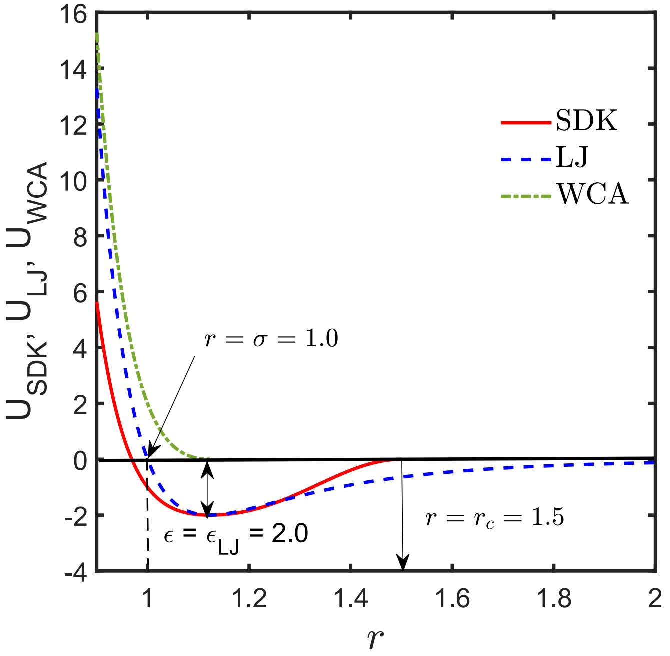


FIG. S1. (Color online) Comparison between the SDK potential ($U_{\rm SDK}$) and the conventional LJ ($U_{\rm LJ}$) and WCA ($U_{\rm WCA}$) potentials as a function of the radial distance, $r$, for well depths $\epsilon = \epsilon_{\rm LJ} = 2.0$, $\sigma = 1$, and $r_c = 1.5$ (see text for corresponding values of $\alpha$ and $\beta$).

The constants $\alpha$ and $\beta$ (as discussed in the main text) are determined by applying the two boundary conditions, namely, $U_{\rm SDK} = 0$ at $r = r_c$, and $U_{\rm SDK} = -\epsilon$ at $r = 2^{1/6}\sigma$. Based on these two boundary conditions, $\alpha$ and $\beta$ are calculated by solving the following set of equations,

$$2^{1/3}\alpha + \beta = \pi \tag{4}$$

$$\left(\frac{r_c}{\sigma}\right)^2 \alpha + \beta = 2\pi \tag{5}$$

In Appendix A of the main text it was shown how the value of $\epsilon_{bb}$ at the $\theta$-point can be estimated by plotting the ratio $R_g^2/(N_b - 1)$ versus $\epsilon_{bb}$ for different chain lengths, $N_b$, and finding the point of intersection at which curves for different values of $N_b$ intersect.[2,3] With the cut-off radius set to $r_c = 1.5\,\sigma$, the $\theta$-point for a homopolymer chain with beads connected by FENE springs having a maximum stretchable length of ${Q_0}^2 = 50.0$, is found to be $\epsilon_{bb} = 0.72$ as shown in Fig. S2. This is in contrast to the value of $\epsilon_{bb} = 0.45$ obtained for $r_c = 1.82\,\sigma$, as was demonstrated in Appendix A. The reasons for the unsuitability of

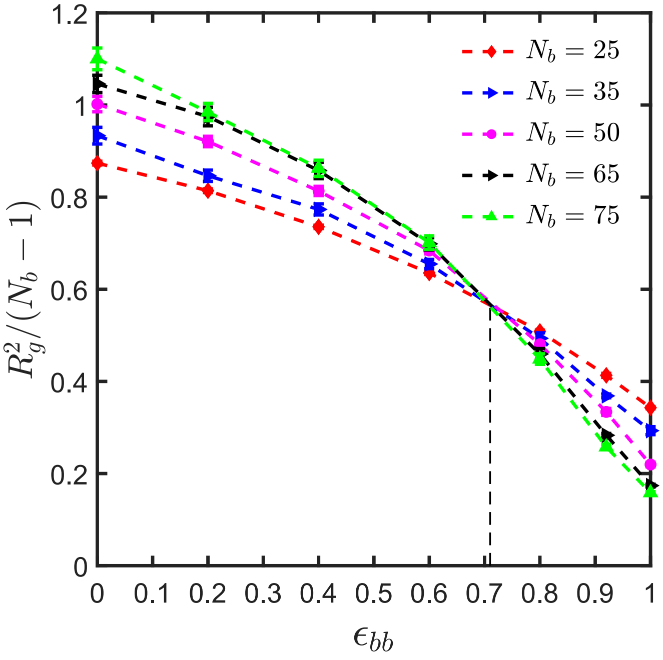


FIG. S2. (Color online) The ratio $R_g^2/(N_b - 1)$ as a function of the well depth of the SDK potential, $\epsilon_{bb}$, used to estimate the $\theta$-point for the cutoff radius $r_c = 1.5\sigma$. The symbols represent simulation data and the dotted lines are drawn to guide the eye. The $\theta$-point is estimated as the intersection of all the curves and leads to $\epsilon_{bb} = 0.72$.

using $r_c = 1.5\,\sigma$ are discussed below.

With increasing values of $\epsilon_{bb}$ beyond $\epsilon_{bb} = 0.72$, the chain begins to collapse due to decreasing solvent quality. In the limit of a poor solvent, linear polymer chains obey the scaling law $R_g \sim (N_b - 1)^{1/3}$, indicating that the chains are space filling. Fig. S3 (a) studies the chain length dependence of $R_g^2$ for various well depths $\epsilon_{bb}$. For $\epsilon_{bb} = 0$ (the athermal limit) and $\epsilon_{bb} = 0.72$ (the $\theta$-point), the expected power law exponents of 1.2 and 1.0, respectively, are observed. For intermediate values in the crossover regime, $0 < \epsilon_{bb} < 0.72$, one expects, strictly speaking, a curve beginning with slope 1 at small values of $N_b$, and gradually increasing to 1.2 for asymptotically long chains. However, for the fairly short chains studied here, this curvature is very hard to observe; instead the data can be well described in terms of an effective exponent, whose variation with $\epsilon_{bb}$ is shown in Fig. S3 (b). An analogous crossover from a slope of 1.0 to (2/3) is expected as the well depth is increased beyond the $\theta$ value of 0.72, with the effective exponent remaining at (2/3) for sufficiently large $\epsilon_{bb}$. However, as can be seen from Figs. S3 (a) and (b), the “asymptotic” slope at

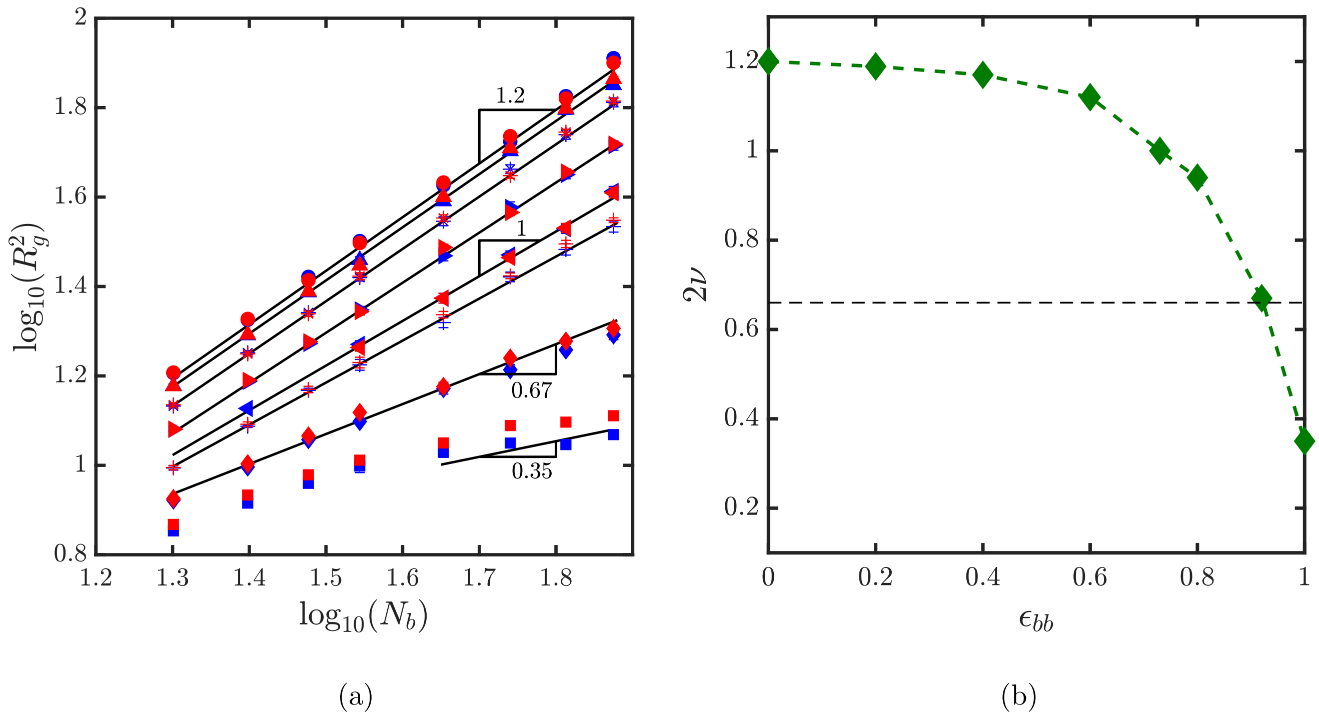


FIG. S3. (Color online) (a) The mean-squared radius of gyration as a function of the number of beads in a chain. The blue-coloured symbols are for different values of well-depth, $\epsilon_{bb}$, in the absence of hydrodynamic interactions. ● $\epsilon_{bb} = 0$, ▲ $\epsilon_{bb} = 0.2$, $*$ $\epsilon_{bb} = 0.4$, ▶ $\epsilon_{bb} = 0.6$, ◀ $\epsilon_{bb} = 0.72$, $+$ $\epsilon_{bb} = 0.8$, ◆ $\epsilon_{bb} = 0.92$ and ■ $\epsilon_{bb} = 1$. The same symbols are used with a red colour for simulations with hydrodynamic interactions. The straight lines are of slope $2\nu$ at different values of $\epsilon_{bb}$. (b) Effective exponent $2\nu$ versus the well-depth, $\epsilon_{bb}$, for cutoff radius $r_c = 1.5\,\sigma$.

$\epsilon_{bb} = 1$ seems to be only 0.35, which is obviously unphysical, if interpreted as an asymptotic scaling law. We can only speculate here about the reasons for this behaviour — since we were able to "cure" the problem without a detailed investigation, we did not attempt to analyse it in depth. However, a few observations may be made.

Firstly, Fig. S3 (a) shows clearly that the data at $\epsilon_{bb} = 1$ are hampered by equilibration problems. This becomes obvious via the comparison of data accumulated with and without hydrodynamic interactions, which, as static averages, must be identical if strict thermal equilibrium and sufficient sampling is achieved. Secondly, it has already been pointed out in Soddemann, Dünweg, and Kremer[1] that the SDK potential with $r_c = 1.5\,\sigma$ has a propensity to induce crystallisation, i.e., highly ordered structures. It is then quite conceivable that the

growth of a highly collapsed globule with chain length occurs essentially in a layer-by-layer fashion, which would then give rise to a fairly abrupt increase of $R_g^2$ as soon as a new layer begins to be populated. The small slope of 0.35 that we observe in Fig. S3 (a) may then perhaps be part of a quasi-plateau that corresponds to oscillations that are added on top of the leading $N^{2/3}$ behaviour.

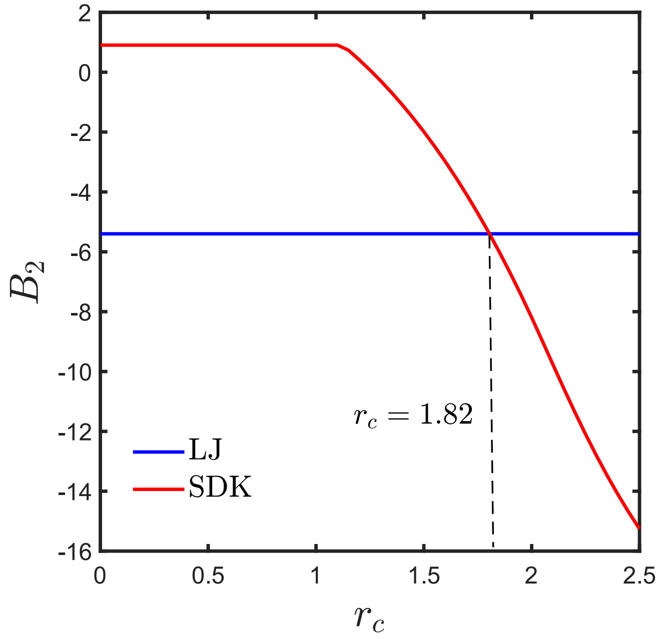


FIG. S4. (Color online) The second virial coefficient $B_2$ of the SDK potential, compared with the corresponding value for the LJ potential, as a function of the cutoff radius, $r_c$, for well-depths $\epsilon_{bb} = \epsilon_{\rm LJ} = 1.0$, and $\sigma = 1$.

Prompted by our experience with using a simple Lennard-Jones potential in analogous studies of collapsing polymer chains,[4] which did not exhibit this problem, we attempted to solve it by modifying the SDK potential such that it would mimic more closely the attributes of the Lennard-Jones potential. In practice, we adjusted the range of the SDK potential $r_c$ by requiring that, for $\epsilon_{\rm LJ} = \epsilon_{bb} = 1$ and $\sigma = 1$, both potentials give rise to the same value of the second virial coefficient given by the integral[5]

$$B_2 = \int_0^\infty 2\pi r^2 (1 - \exp[-U(r)/k_B T])\, dr. \qquad (6)$$

Matching this value with the corresponding LJ value results in $r_c = 1.82\,\sigma$ (see Fig. S4), for which $\alpha = 1.5306333121$ and $\beta = 1.213115524$. In view of the remarks made earlier, it is

well conceivable that such a smoother potential will exhibit less pronounced oscillations or perhaps none at all.

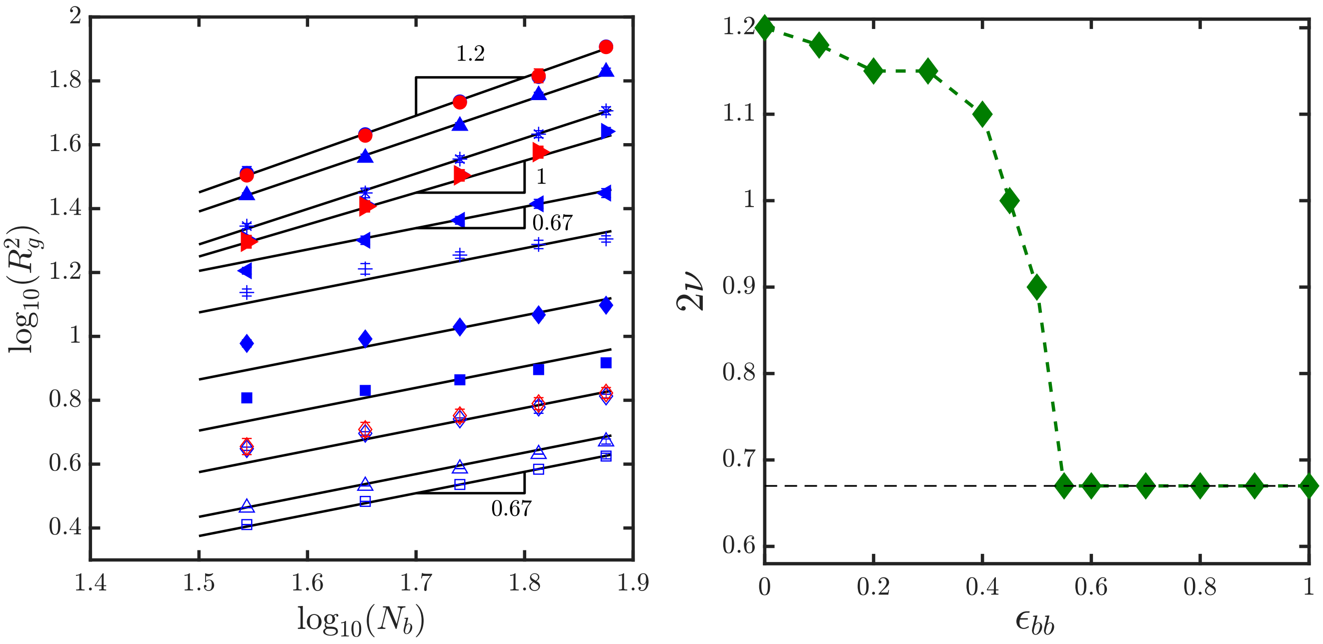


(a)

(b)

FIG. S5. (Color online) (a) The mean-squared radius gyration versus number of beads in a chain. The blue-coloured symbols are for different values of well-depth, $\epsilon_{bb}$, in the absence of hydrodynamic interactions. • $\epsilon_{bb} = 0$, ▲ $\epsilon_{bb} = 0.2$, $*$ $\epsilon_{bb} = 0.4$, ▶ $\epsilon_{bb} = 0.45$, ◀ $\epsilon_{bb} = 0.55$, $+$ $\epsilon_{bb} = 0.6$, ♦ $\epsilon_{bb} = 0.7$ and ■ $\epsilon_{bb} = 0.8$, ◊ $\epsilon_{bb} = 1$, △ $\epsilon_{bb} = 2$ and □ $\epsilon_{bb} = 3$. The same symbols are used with a red colour for simulations with hydrodynamic interactions. The straight lines are of slope $2\nu$ at different values of $\epsilon_{bb}$. (b) Exponent $2\nu$ versus the well-depth, $\epsilon_{bb}$, at cutoff radius $r_c = 1.82\,\sigma$.

As seen in Fig. S5 (a), the effective exponent shows a gradual decrease from 1.2 at $\epsilon_{bb} = 0$ to 0.67 at $\epsilon_{bb} = 0.55$, and it remains constant at 0.67 well beyond $\epsilon_{bb} = 0.55$, as shown in Fig. S5 (b). The values of the mean-squared radius of gyration, $R_g^2$, are reproduced with HI for $\epsilon_{bb} = 0$, 0.45 and 1.0, for different chain lengths and found to be consistent with the results without HI (as seen in Fig. S5 (a)). All the results reported in the current work with the SDK potential are consequently for $r_c = 1.82\,\sigma$.

## References

[1]T. Soddemann, B. Dünweg, and K. Kremer, "A generic computer model for amphiphilic systems," EPJ **6**, 409–419 (2001).

[2]M. O. Steinhauser, "A molecular dynamics study on universal properties of polymer chains in different solvent qualities. Part I. A review of linear chain properties," J. Chem. Phys. **122**, 094901 (2005).

[3]S. Huissmann, R. Blaak, and C. N. Likos, "Star polymers in solvents of varying quality," Macromolecules **42**, 2806–2816 (2009).

[4]T. T. Pham, B. Dünweg, and J. R. Prakash, "Collapse dynamics of copolymers in a poor solvent: Infuence of hydrodynamic interactions and chain sequence," Macromolecules **43**, 10084–10095 (2010).

[5]M. Rubinstein and R. H. Colby, *Polymer Physics* (Oxford University Press, 2003).
